# Supplementary material for: Impact of the sodium and calcium chlorides uptake on the interfacial behavior of ice: premelting, structure, and dynamics
Source: arXiv:2512.21929 source file (2025-12-26)
Supplement: Supplementary file 1 [file suppinfo.pdf]

# Supporting Information: Impact of the sodium and calcium chlorides uptake on the interfacial behavior of ice: premelting, structure, and dynamics.

Łukasz Baran, Luis G. MacDowell

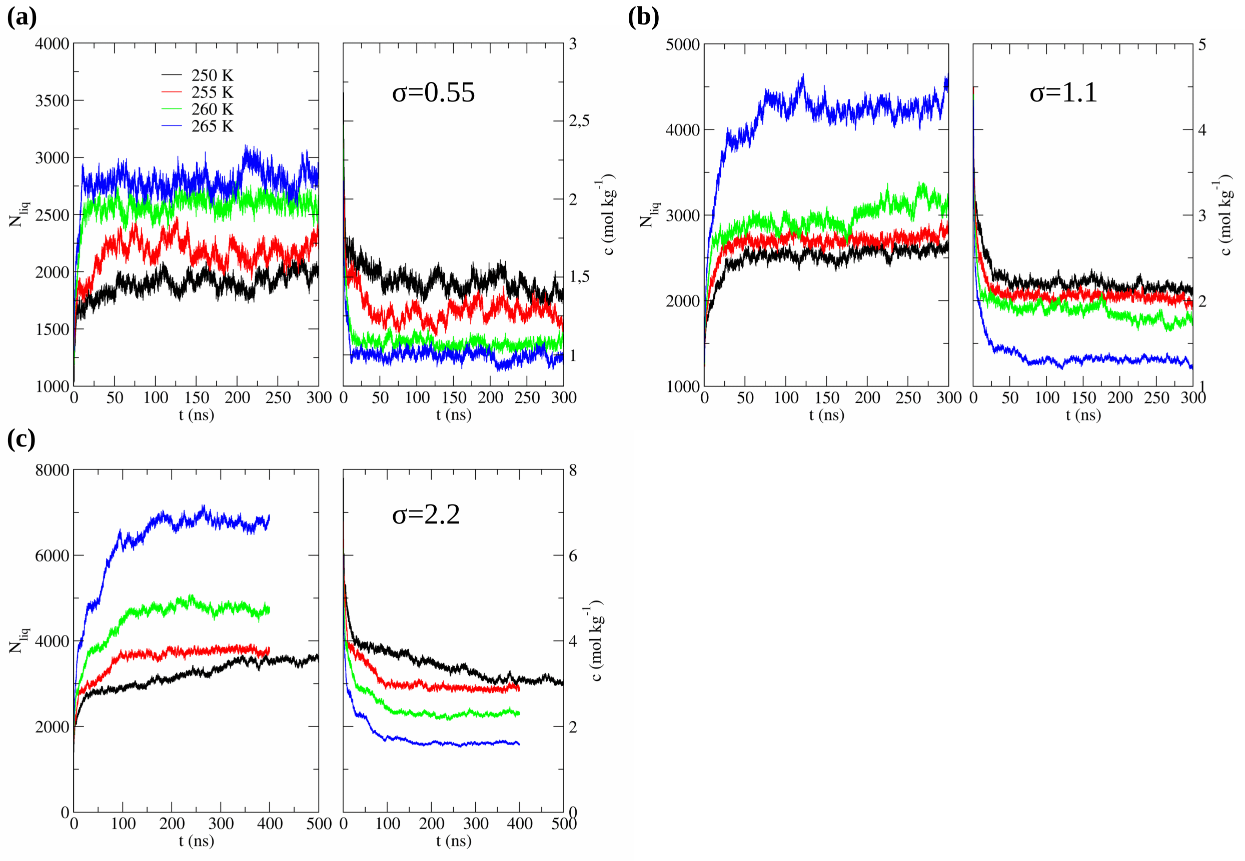


Figure S1: Time evolution of the number of liquid-like molecules (left panels) and the concentration of the NaCl brine formed at the ice-vapor interface (right panels) for four different temperatures and three surface coverages.

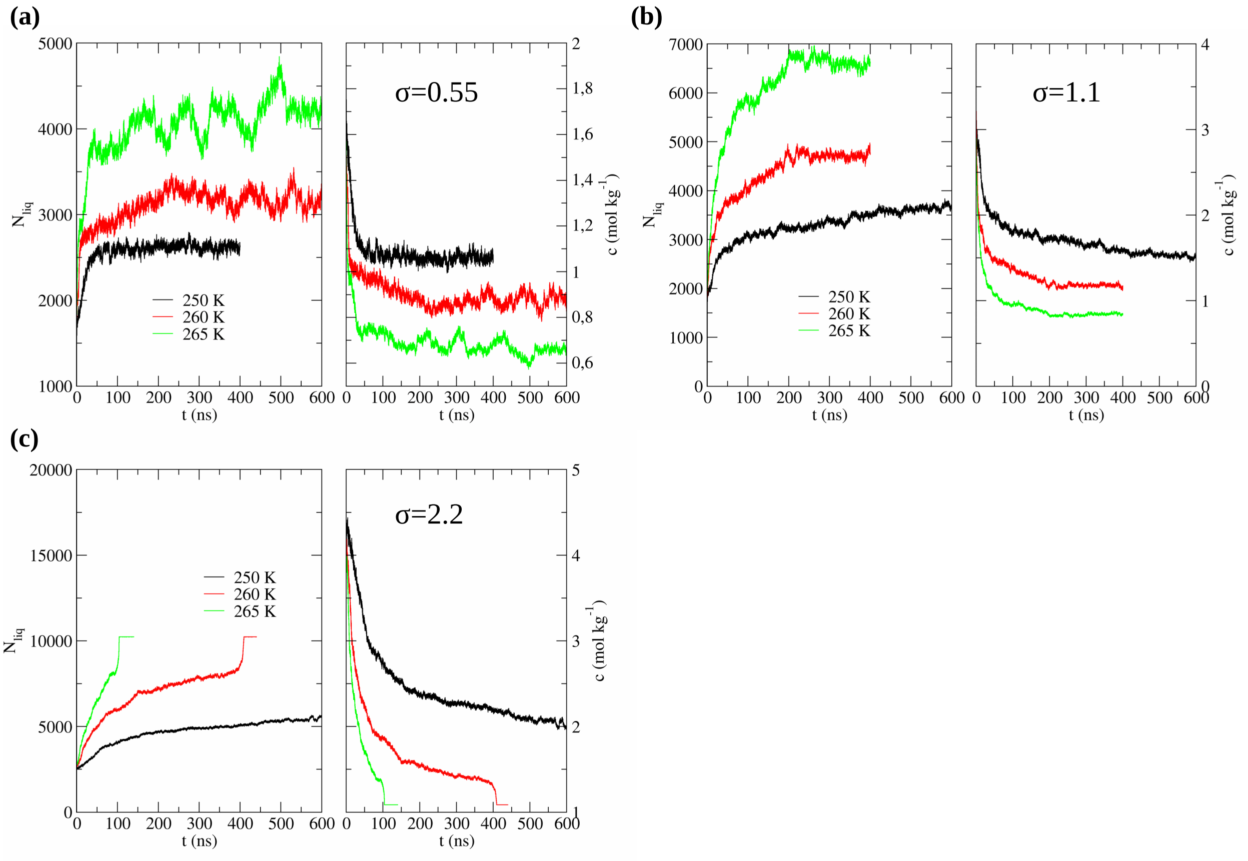


Figure S2: Time evolution of the number of liquid-like molecules (left panels) and the concentration of the $CaCl_2$ brine formed at the ice-vapor interface (right panels) for three different temperatures and three surface coverages.
